# Supplementary material for: Generation and imaging of magnetoacoustic waves over millimetre distances
Source: arXiv:1908.11674 source file (2019-12-31)
Supplement: Supplementary file 1 [file Supp_Notes_magnetoacousti_waves.pdf]

Supplementary Material

# Generation and imaging of magnetoacoustic waves over millimetre distances

Blai Casals[1,a], Nahuel Statuto[1,2], Michael Foerster[3], Alberto Hernàndez-Mínguez[4], Rafael Cichelero[1,b], Peter Manshausen[1], Ania Mandziak[3], Lucía Aballe[3], Joan Manel Hernàndez[2], Ferran Macià[1,2]

[1]Institut de Ciència de Materials de Barcelona (ICMAB-CSIC), Campus UAB, 08193 Bellaterra, Spain
[2]Department of Condensed Matter Physics, University of Barcelona, 08028 Barcelona, Spain
[3]ALBA Synchrotron Light Source, 08290 Cerdanyola del Vallès, Spain
[4]Paul-Drude-Institut für Festkörperelektronik, Hausvogteiplatz 5-7, 10117 Berlin, Germany
[5]Instituto de Química Física "Rocasolano", Madrid, 28006, Spain

[*]ferran.macia@ub.edu
[a]now at Cambridge
[b]now at Department of Physics, University of Gothenburg, 412 96 Gothenburg, Sweden

# Ferromagnetic resonance spectroscopy

In order to determine the dynamic magnetic properties of our nickel thin films we conducted FMR spectroscopy with frequencies ranging from 0.1 to 6 GHz as a function of the applied field at room temperature. We studied extended films of nickel deposited in Si/$SiO_x$ substrates deposited together with the films studied for magnetoacoustic waves. To record the weak signals of the thin magnetic layer we used a coplanar waveguide (CPW) with a flat signal transmission within the used frequency range. The absorption signal was recorded by sweeping the magnetic field at constant frequency with the sample mounted 'flip-chip' on the CPW [1]. Figure S1**A** shows the frequency dependence of the transmission signal in the CWG as a function of the applied field. The curves are shifted vertically for visual purposes. We observe the appearance of resonance peaks at frequencies above 1.6 GHz whereas a single peak centered at zero field appears at lower frequencies. Figure S1**B** shows the frequency as a function of the resonance field extracted from data in Fig. 1**A**. The applied magnetic field was in the film plane and for a magnetic thin film with in-plane uniaxial anisotropy and magnetized to saturation along the easy axis, the Kittel FMR frequency $f$ as a function of a static external field, $H$, may be written as

$$2\pi f = \mu_0 \gamma \sqrt{(H + H_K)(H + H_K + M_S)},$$

where $\gamma$ is the gyromagnetic ratio, $M_s$ is the saturation magnetisation and $\mu_0 H_K = \frac{2K_U}{M_S}$ is the uniaxial anisotropy field ($K_U$ is the magnetic anisotropy). The fitting is compatible with an existing anisotropy in the applied field direction of about $K_U \approx 300$ J/m$^3$.

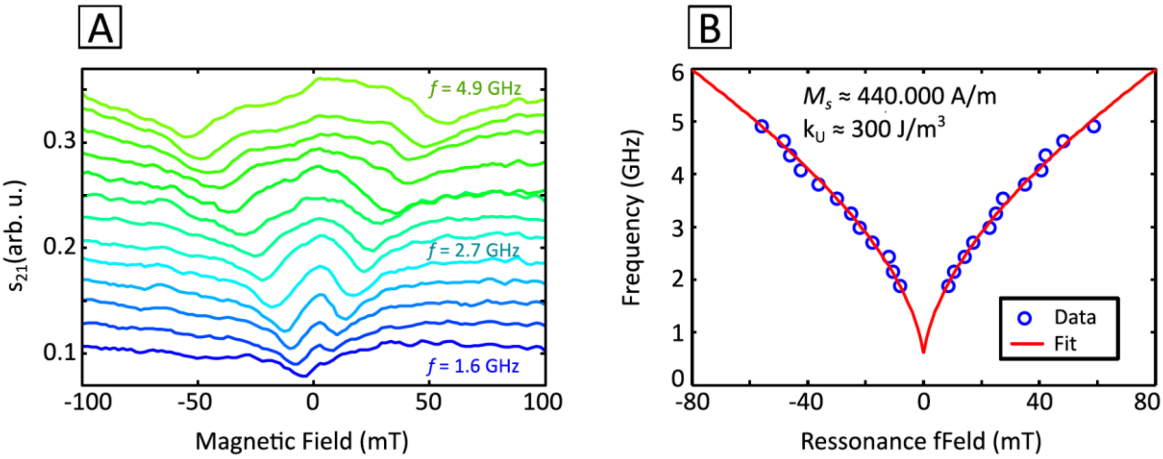


Figure S1. Experimental FMR spectrum for a 10 nm nickel thin film deposited on $LiNbO_3$. In **A** an in plane field is swept from negative to positive values and the transmission parameter of the CWG, $s_{21}$, is recorded. In **B** we plot the resonance fields and frequencies from **A**, fitted using a macrospin model.

# Micromagnetic simulations.

We modeled the dynamic anisotropy variations in the Ni thin film with micromagnetic simulations using the open-source MuMax$^3$ code [2] on a graphics card with 2048 processing cores. We considered a two-dimensional layer and integrated the Landau-Lifshitz-Gilbert equation to describe the magnetisation dynamics. Thermal effects were neglected. The parameters of the magnetic layer, a nickel film, were taken the following: saturation magnetisation $M_s$ = 490 × 10$^3$ Am$^{-1}$, Gilbert damping constant $\alpha$ = 0.03, and exchange constant $A$ = 5 × 10$^{-12}$ Jm$^{-1}$. We considered a time and spatially varying uniaxial anisotropy induced by the SAW with a value $k_{\mathrm{ME}}$ = 600 Jm$^{-3}$. We also introduced in the simulations a fixed uniaxial anisotropy in the $x$ direction with values $k_x$ = 0-1200 Jm$^{-3}$ in addition to the SAW induced time and space varying anisotropy. The simulated area corresponds to a full wavelength with boundary condition in order to avoid shape anisotropy effects.

We note that the SAW induced anisotropy variations produce an essentiality different effect on the magnetisation compared with an oscillating magnetic field (as in FMR experiments). The anisotropy defines a direction but with no preference between signs—either positive or negative. As a consequence, an applied field perpendicular to the varying anisotropy produces no effect on the magnetisation (there is no clear preferred direction for the magnetisation to align with). When the applied field is in the same direction of the varying anisotropy, there is no effect either, which is also the case for oscillating magnetic fields. In summary, we must set the applied magnetic field with certain angle (between 0 and 90 deg.) with respect to the SAW induced anisotropy—we showed 59 deg. in the main manuscript and we also show experimental data at other angles in the following section.

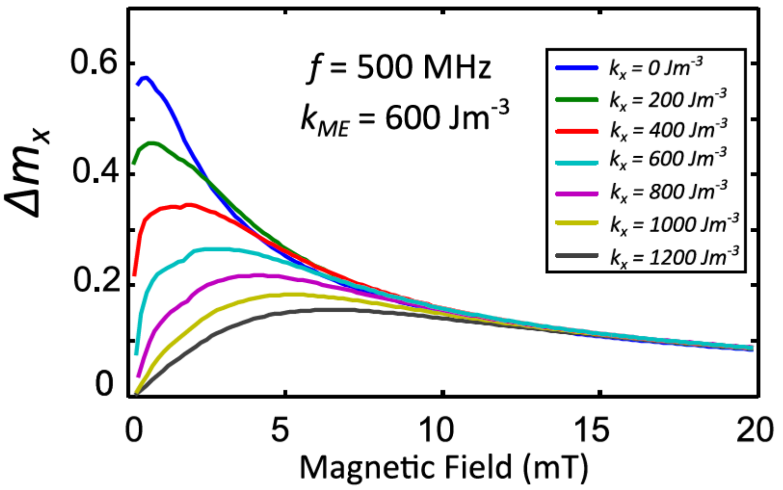


Figure S2. Magnetic response of a Nickel thin film upon SAW excitation as a function of the applied magnetic field (overall amplitude of the magnetisation along the $x$ axis, $\Delta m_x$). An oscillating anisotropy term ($f$ = 500 MHz and $\lambda$ = 8 µm) along the $x$ direction is considered with a value $k_{ME}$ = 600 Jm$^{-3}$. The plot compares different uniaxial magnetic anisotropies along the $x$ direction. The applied field forms an angle of 59 deg

We applied a magnetic field with an angle of 59 deg. with respect to the SAW propagation direction and swept the field from a positive value of 20 mT down to zero while recording the magnetic response of the simulated area. Figure S2 shows the magnetic response variation in the $x$ component, $\Delta m_x$, as a function of the applied magnetic field for a SAW induced time and space varying anisotropy. We compare at a frequency of 500 MHz and a wavelength of 8 µm (same values as most of the data in the main manuscript) the effect of an additional induced uniaxial anisotropy in the $x$ direction, $k_x$. We can see that for $k_x$ = 0 the amplitude of the magnetic response increases as the magnetic field goes to zero showing a small peak below 1 mT, which is caused by the resonance frequency. As the uniaxial anisotropy increases (we use values up to 1200 Jm$^{-3}$), there is a

competition between the torque made by the applied field, the torque made by the uniaxial magnetic anisotropy, and the torque produced by the SAW on the ferromagnet's magnetisation. At large applied fields, the ferromagnet's magnetisation aligns with the field; at zero applied field, the magnetisation aligns with the uniaxial anisotropy along the *x* direction. In Fig. S2 we observe that when the uniaxial anisotropy increases the magnetic response goes to zero at zero applied field (as well as at large fields) and the maximum variation shifts towards larger field values.

Next, we investigated the effect of a forced wavelength on the magnetic excitation. We note that SAWs have a dispersion relation, which sets a particular wavelength for each excitation frequency, $f = v_{SAW}/\lambda$, where $v_{SAW}$ is the speed of sound in $LiNbO_3$. However, we find it instructive to compare micromagnetic simulations with a fixed frequency and a varying wavelength. In Figure S3 we plotted the magnetic response variation as a function of the applied magnetic field for a SAW induced time and space varying anisotropy. We compare different wavelengths at a fixed frequency of 500 MHz with also a fixed uniaxial anisotropy $k_x$ = 800 $Jm^{-3}$. Figure S3**A** shows the oscillation in the magnetisation projected on the *x* axis (this is the quantity observed with XMCD). Figure S3**B** shows the overall amplitude of the magnetisation along the *x* axis. We observe that the case with no spatially varying anisotropy (blue curve) shows a peak around 3 mT corresponding to the maximum effect of the SAW. The effect of a forced spatial dependence (a wavelength) of the oscillating SAW-induced anisotropy is a reduction of the amplitude of the excitation together with a slight shift of the maximum (the relevant magnetic interactions such as exchange and dipolar fields increase with decreasing wavelength).

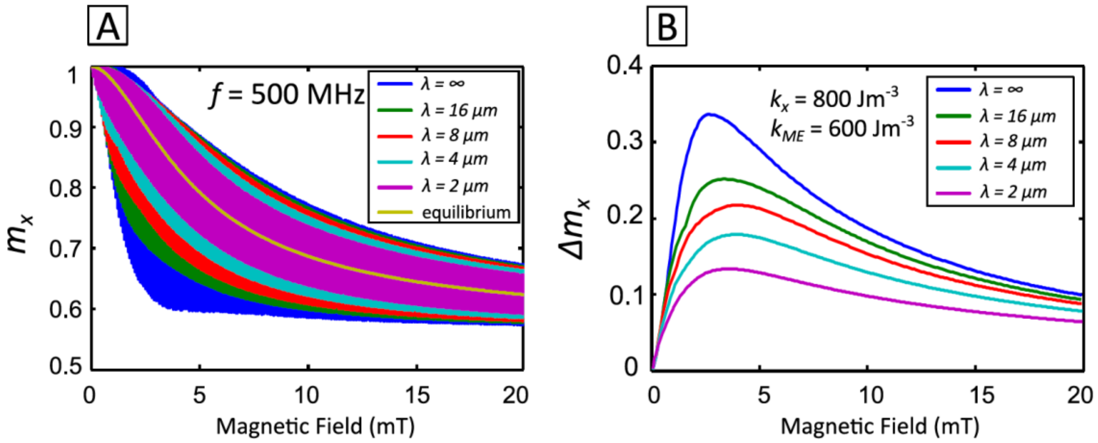


Figure S3. Magnetic response of a Nickel thin film upon SAW excitation as a function of the applied magnetic field. We impose a uniaxial anisotropy in the x direction with a value $k_x$ = 800 $Jm^{-3}$ and an oscillating term (*f* = 500 MHz) induced by the SAW with value $k_{ME}$ = 600 $Jm^{-3}$. We compare different wavelengths of SAW induced anisotropy with values 2-16 μm and also the spatially uniform case. **A** shows the oscillation in the magnetisation projected to the *x* axis (this is the quantity observed with XMCD). **B** shows the overall amplitude of the magnetisation along the *x* axis. The applied field forms an angle of 59 deg. with the SAW propagation (along *x*).

# Additional XPEEM and XMCD images of acoustic spin waves

In this section we provide additional images of the acoustic spin waves taken at 500 MHz at different sample locations and with different angles of the applied field.

First, we provide two sets of measurements of the hybrid Ni/$LiNbO_3$ with the applied field at 59 deg. with respect to the SAW propagation at two different positions of the sample. The first set of measurements shown in Fig. S4 has the Nickel thin film in the lower part and the $LiNbO_3$ at the top. There is no non-magnetic metallic part to provide a reference and thus we cannot extract precise values on the magnetisation variation as we did in the set shown in the main manuscript. The magnetisation signal decreases with increasing field and eventually vanishes. We notice that SAW is also visible in the XMCD signals because the sample was not fully thermalized and a small variation in the conductivity of the sample produced different image contrast (and then the SAW component in the $LiNbO_3$ does not fully cancel when subtracting images with different helicities).

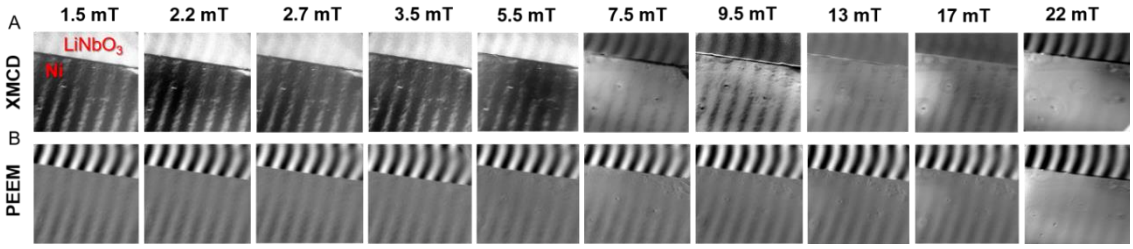


Figure S4. In **A**, XMCD images as a function of the applied magnetic field from 1.5 to 22 mT. In **B** images at the same fields obtained by subtracting two PEEM images with opposite SAW phases. The applied field has an angle of 59 deg. with respect to the SAW propagation direction.

The second set of measurements corresponds to the images shown in the main manuscript. Figure S5 shows an extended set of images with all measured fields. The contrast in all images is normalized.

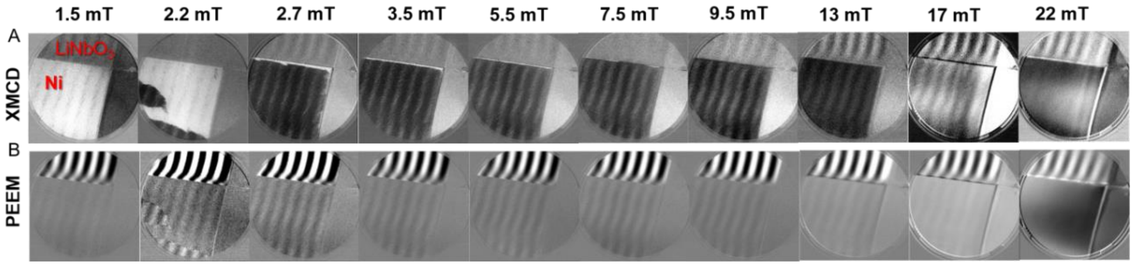


Figure S5. In **A**, XMCD images as a function of the applied magnetic field from 1.5 to 22 mT. In **B** images at the same fields obtained by subtracting two PEEM images at opposite SAW phases. The applied field has an angle of 59 deg. with respect to the SAW propagation direction.

Next we rotated our sample by 90 degrees so that the applied field forms an angle of 30 deg. with the SAW propagation direction. Images in Fig. S6 show similar magnetisation patterns and field dependence. We notice that the magnetic domain formation during magnetisation reversal varies from the previous image sets, which can be due to the uniaxial anisotropy of the film (which now has a different relative angle with the applied field).

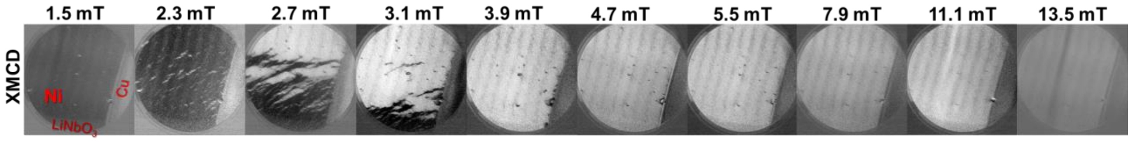


Figure S6. XMCD images as a function of the applied magnetic field from 1.5 to 13.5 mT. The applied field has an angle of 30 deg. with respect to the SAW propagation direction.

An applied field along the SAW propagation direction causes no effect on the ferromanget's magnetisation (the magnetoelastic induced anisotropy is parallel to the magnetisation and there is no resulting torque). Figure S8 shows a set of images with the applied magnetic field parallel to the SAW propagation direction. The contrast inversion between Fig S7**A** and Fig. S7**C** as well as the domains in Fig. S7**B** demonstrate that we are sensitive to the magnetisation and the image in Fig. S7**D**, obtained by subtracting two images at opposite SAW phases, confirms the presence of the SAW.

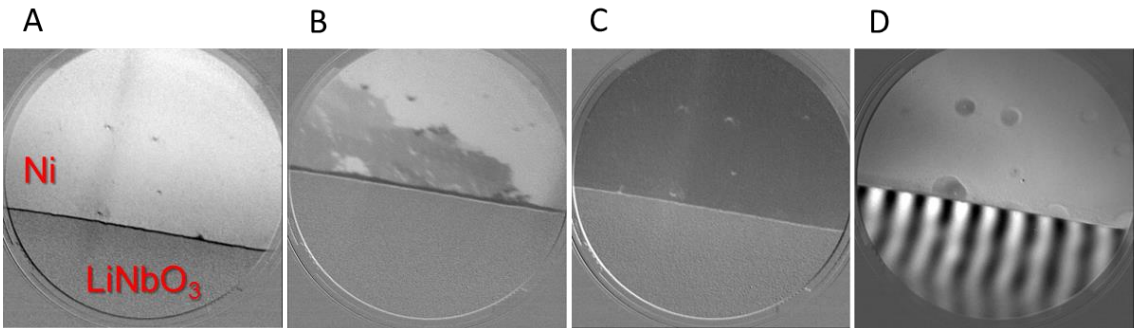


Figure S7. XMCD images of the Nickel thin film (top) at zero applied field after saturation in positive (**A**) and negative (**C**) and a demagnetisation process (**B**). We observe in A the Nickel is white whereas in C it is black compared with the $LiNbO_3$ (lower part of the image). Image **B** shows magnetic domains. Image **D** is a XPEEM image highlighting the SAW. No contrast in the Nickel film is observed at any applied magnetic field.

# Video description

The video shows a sequence of images at different phases of an acoustic spin wave when there is a single (top panel) and double (lower panel) SAW excitation. In the first case a propagating magnetisation wave is observed whereas in the second case we have a standing magnetisation wave. We notice that to obtain an interference pattern with strongly dominating standing wave we need to fine tune both the amplitude and the phases of the two SAW generators [3]. A Snapshot of the video is shown in Fig S8.

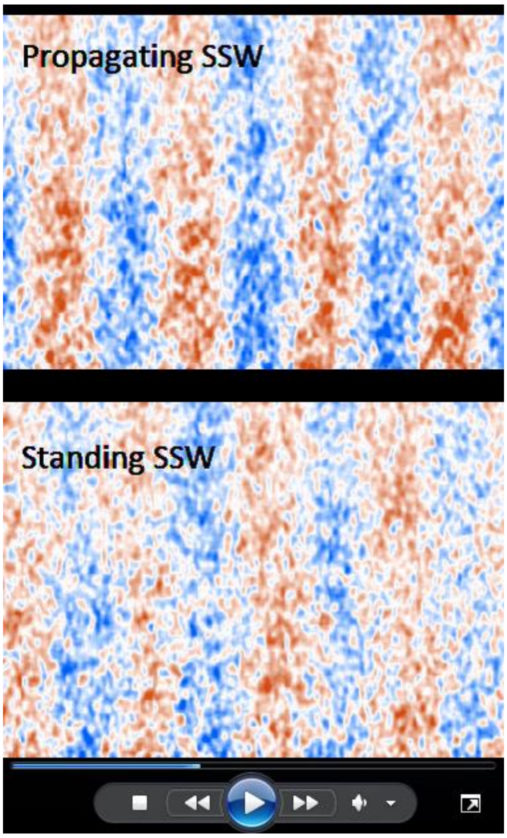


Figure S8. Snapshot of a video showing a propagating (top) and a standing (bottom) magnetoacoustic wave.

## SUPPLEMENTARY REFERENCES

[1] F. Macià, P. Warnicke, D. Bedau, M.-Y.Im, P.Fischer, D.A. Arena and A.D. Kent. J. Magn. Magn. Mater. **324**, 3629 (2012)

[2] A. Vansteenkiste, J. Leliaert, M. Dvornik, M. Helsen, F. Garcia-Sanchez, and B. V. Waeyenberge, AIP Advances **4**, 107133 (2014).

[3] M. Foerster, et al., Journal of Synchrotron Radiation 26, 184 (2019).
